# Supplementary material for: Topological protection breakdown: a route to frustrated ferroelectricity
Source: arXiv:2406.14646 source file (2025-09-30)
Supplement: Supplementary file 1 [file Supercrystal_Vortex_Supplementary.pdf]

# Supplemental Material: Frustrated ferroelectricity from interlocked topological defects

Ludovica Falsi[1,2], Pablo Villegas[2,3],[*] Tommaso Gili[4], A. J. Agranat[5], and E. DelRe[1,6]
[1]*Dipartimento di Fisica, Università di Roma "La Sapienza", 00185 Rome, Italy*
[2]*Enrico Fermi Research Center (CREF), Via Panisperna 89A, 00184, Rome, Italy*
[3]*Instituto Carlos I de Física Teórica y Computacional, Universidad de Granada, Granada, Spain*
[4]*Networks Unit, IMT Scuola Alti Studi Lucca, Piazza San Francesco 15, 55100- Lucca, Italy.*
*The Institute of Applied Physics, The Hebrew University, Jerusalem 91904, Israel and*
[5]*Institute for Complex Systems, National Research Council, Rome 00185, Italy*

## CONTENTS

Two dimensional squared lattices 2

LRG analysis of the multi-scale lattice 3

Microscopic counting of spontaneous polarization states 3

Temporal variability in the metastable phase 5

Snapshots of the different phases 5

2D Fourier transform analysis 6

Experimental set-up 7

Percolation analysis of SC structures 8

References 9

## TWO DIMENSIONAL SQUARED LATTICES

Here, we have synthesized in Fig. 1 different microscopic configurations of a hypothetic vortex structure arranged in a 2D simple squared lattice. We have selected different regular vortex and antivortex configurations to evidence the impossibility of creating an organized, ordered structure (from the point of view of the microscopic system configurations). The first scenario involves the potential occurrence of an ordered domain consisting of vortex/antivortex patterns: to avoid an unstable configuration, this needs careful inclusion of negative links ensuring some antiferroelectric interactions (red lines in Fig. 1(top)). In the second case, we consider the generation of an ordered vortex structure. However, this necessarily involves the emergence of frustrated plaquettes that are excluded by any possible DM-like interaction (Fig. 1(bottom)). Therefore, we can conclude that the simplest topological structure that can sustain an ordered vortex structure under the consideration of DMI is represented by our proposal in the main text.

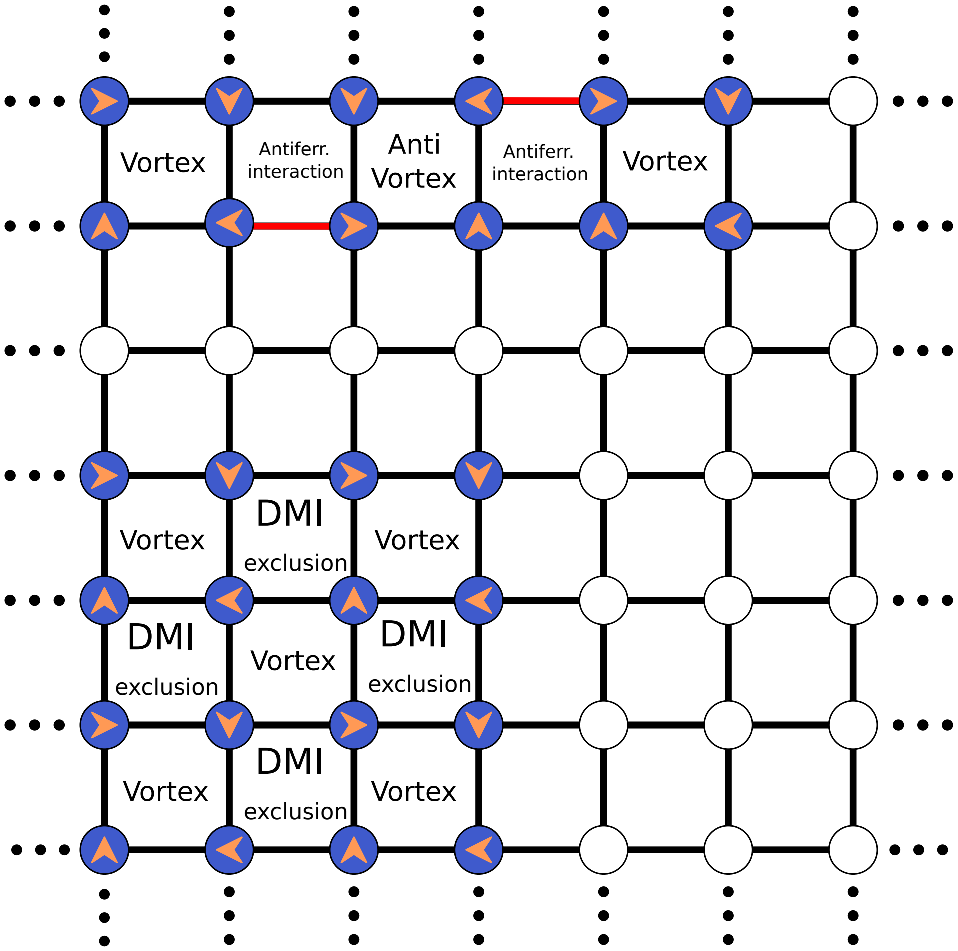


FIG. 1. **Regular 2D lattices**. Sketch of the possible microscopic configurations in a 2D regular lattice. All the different possibilities lead to an unstable system from a microscopic point of view.

## LRG ANALYSIS OF THE MULTI-SCALE LATTICE

To better understand how the SC's multiscale lattice changes at different scales, we employed the methodology of the recently introduced Laplacian Renormalization Group (LRG) [1] to perform successive reductions of the original topological underlying structure, which governs the interactions between mesoscopic polarized regions of the SC. In particular, as shown in Fig. 2, the microscopic scales, which allow the formation of multiple vortices, collapse into single macro-nodes that interact in a simple square lattice in the successive scale, as expected by visual inspection of the 2D lattice.

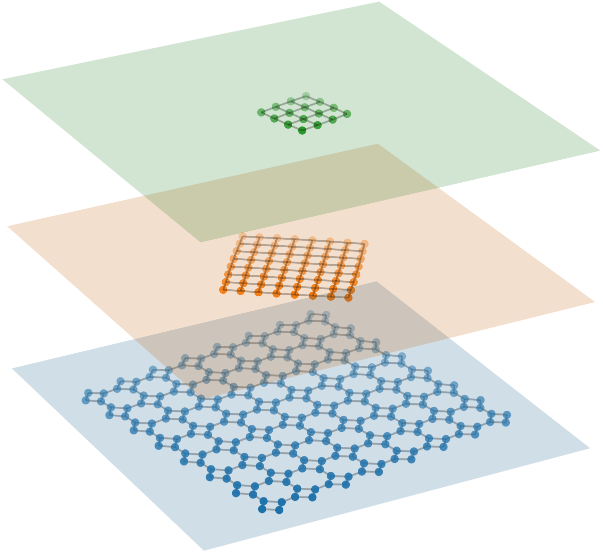

FIG. 2. **LRG transformations.** Lattice reduction from a small system with $N = 256$ nodes to a final network of $N = 16$ nodes. The microscopic scale where vortices are formed collapses, at a coarse-grained scale, into a regular square lattice where each vortex forms a Kadanoff block, as indicated in the main text.

## MICROSCOPIC COUNTING OF SPONTANEOUS POLARIZATION STATES

Here, we analyze different characteristic microscopic configurations using the Hamiltonian presented in the main text to make a precise comparison between the Heisenberg-like energetic term and the DMI term. The microscopic configuration of each dipole is described by:

$$\mathcal{H} = -\sum_{\langle i,j\rangle} J_{ij}\mathbf{p}_i \cdot \mathbf{p}_j + \sum_{\langle i,j\rangle} \mathbf{D}_{ij} \cdot (\mathbf{p}_i \times \mathbf{p}_j) \tag{1}$$

where $\mathbf{p}_i$ are the n-component classical vectors representing local polarizations.

Figure 3 displays the energy sum-over-dipoles of this Hamiltonian for the smallest microscopic scale, $\Lambda_1$, of the SC lattice. Our analysis illustrates how microscopic configurations with aligned dipoles (upper part of Fig. 3) have zero energy for those terms that are different from the Heisenberg one. However, for topological defects like vortices, sinks, and sources, the condition of zero local charge density plays a crucial role in the system. It is important to note that we have reported only a small subset of the total of $4^4 = 256$ possible configurations of the four-dipole states at the $\Lambda_1$-scale level.

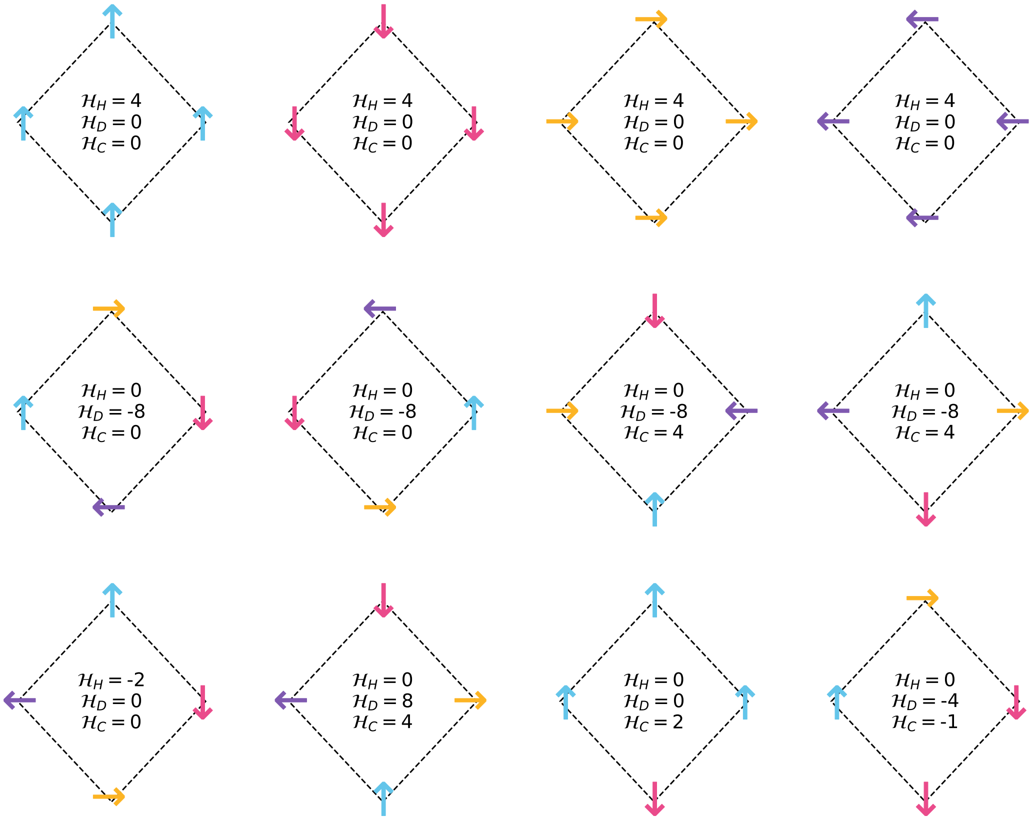


FIG. 3. **Microscopic configurations.** Selected relevant polarization alignments with the corresponding energetic terms. Note that both vortex and sinks/sources form topologically equivalent defects that become forbidden because the term added to each plaquette excludes this microscopic (unphysical situations), leading to zero local charge density.

## TEMPORAL VARIABILITY IN THE METASTABLE PHASE

Figure 4 shows the broad quasi-periodic temporal oscillations of $P$ that characterize the metastable phase.

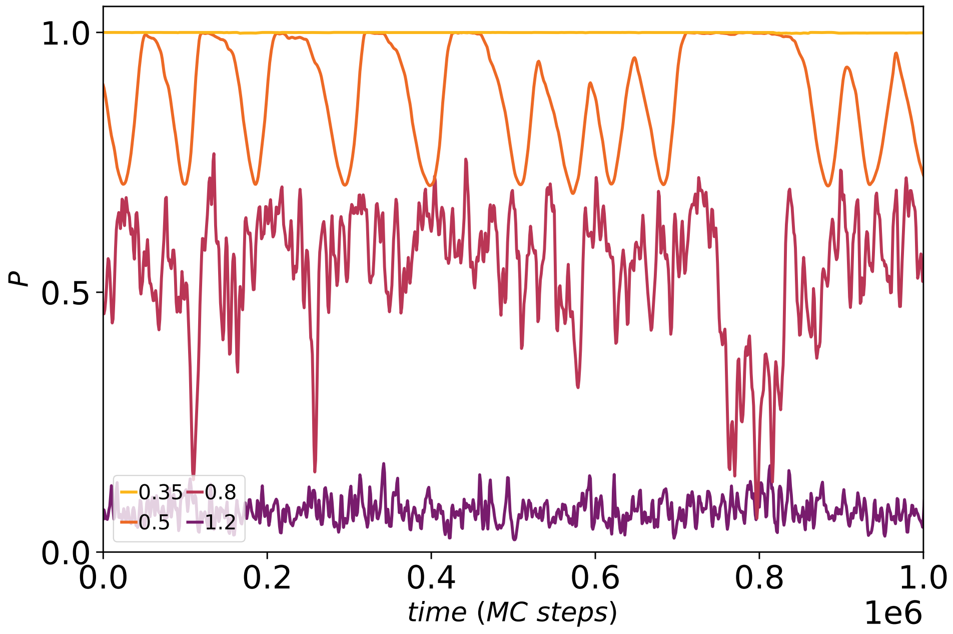


FIG. 4. **Temporal variability.** Polarization order parameter ($P$) as a function of time (in Monte Carlo steps). Different colors represent different values of $T$ (see legend). The broad variability characterizing the metastable phase wildly depends upon the initial conditions for each realization. Parameters: $J/D = 1.4$, $L = 32$.

## SNAPSHOTS OF THE DIFFERENT PHASES

We present several snapshots of the dipole configurations for different phases to complement the main text. These snapshots are reported varying the ratio $J/D$ and the temperature $T$. Fig. 5 (a) illustrates the vortex phase, while Figs. 5 (b), (c) show two metastable distribution of dipoles corresponding to two different temperature on the phase diagram reported in the main text.

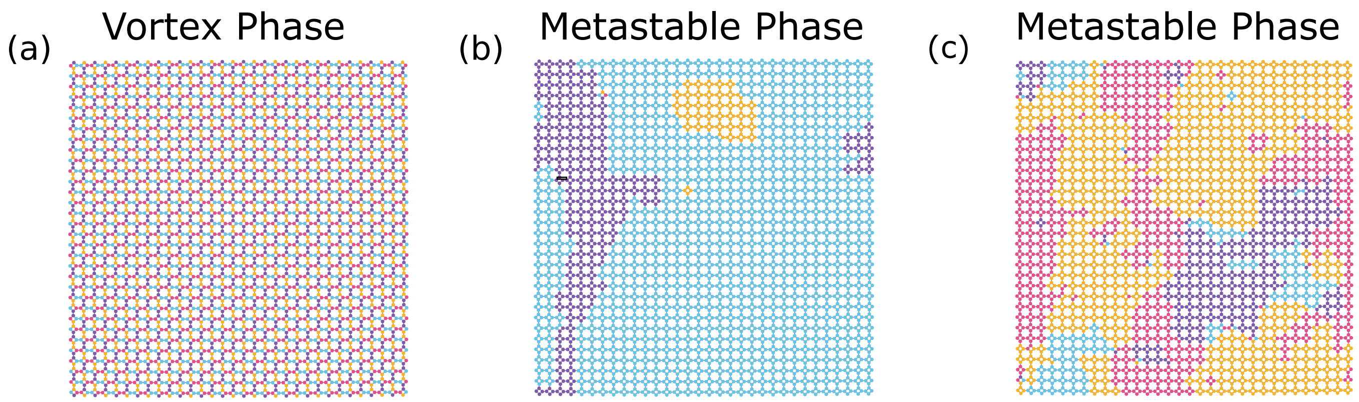


FIG. 5. **Snapshots of several dipole arrangements for different phases. (a)** $J/D = 0.8$, $T = 0.35$, **(b)** $J/D = 1.4$, $T = 0.5$ **and (c)** $J/D = 1.4$, $T = 0.8$. **Parameters:** $L = 32$.

## 2D FOURIER TRANSFORM ANALYSIS

To analyze the 2D vortex structure in Fourier space, we performed spatial analysis of the grayscale vortex pattern generated by the following procedure:

1. We identify the structural effects caused by the underlying lattice by setting all vortices to an 'alpha' channel of $\alpha = 0$. This gives us the regular structure presented in Fig. 6(a).

2. Once we have understood the effects produced by the spatial lattice in Fourier space, we subtract these terms from the original FFT in the vortex phase, as shown in Fig. 6(d). This resulted in the final FFT, where the pure effect of the vortex structure could be safely filtered, as described in the main text.

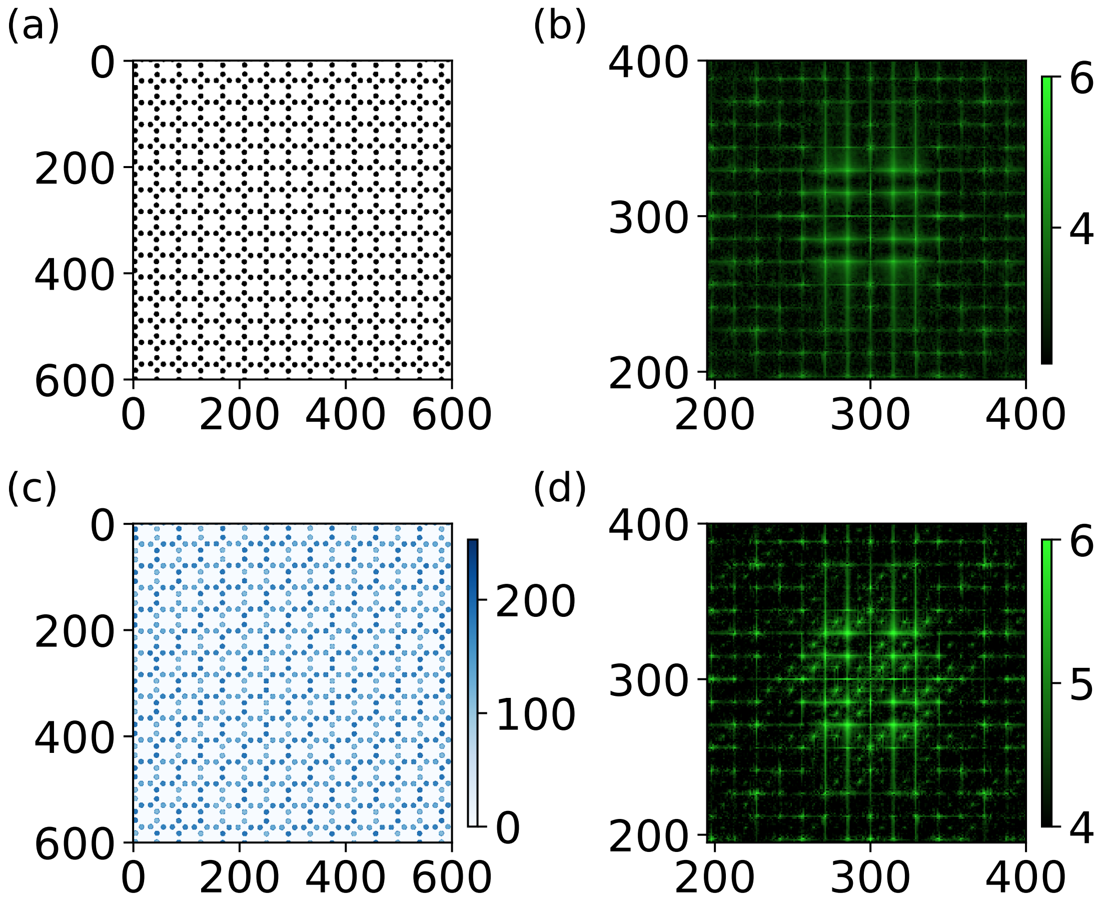


FIG. 6. **2D Fourier analysis.** **(a)** Binarized lattice. **(b)** 2D Fourier transform of the previous 2D lattice. **(c)** 2D lattice with vortex structure encoded in the grayscale values. **(d)** 2D Fourier transform of the corresponding spatial arrangement of dipoles in the vortex phase.

## EXPERIMENTAL SET-UP

The experimental setup is illustrated in Fig. 7. Laser light from a doubled 30 mW Nd:YAG laser (wavelength $\lambda = 2\pi/k_0 = 532$ nm) is made to propagate along the z-axis through the zero-cut KTN:Li crystal sandwiched in between two crossed polarizers (P1 and P2). The sample is biased by a time-constant electric field E along the x-axis. The crystal temperature T is set by a current-controlled Peltier junction in contact with one of the y facets. Light from the crystal output facet is imaged using a moveable spherical lens L1 (of focal length 50mm) onto a CMOS camera.

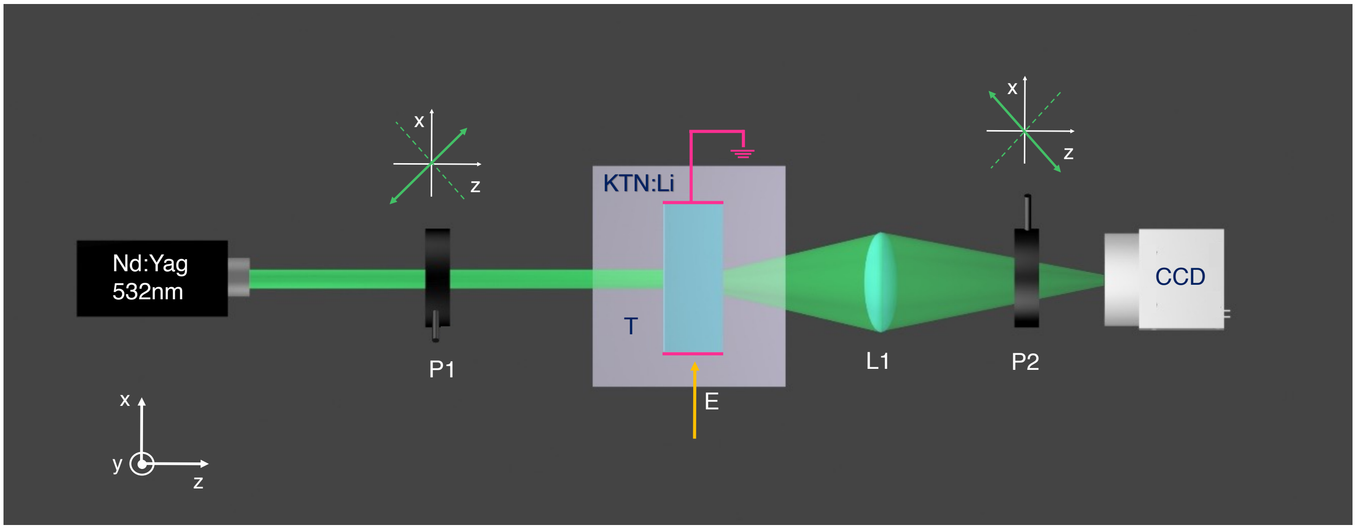


FIG. 7. **Experimental Setup**

## PERCOLATION ANALYSIS OF SC STRUCTURES

Basic phenomenology is reported in Fig. 8, where polarization transmission images through the sample are shown for various temperatures below $T_c$ =294K and different external electric fields $E$. In pure depoled ferroelectrics, random birefringence causes complete depolarization of propagating optical fields, resulting from multiple interferences of random scattered waves. In contrast, light propagating in a SC suffers a GR, where waves travel along the principal axes of the crystal without diffracting, remaining fully polarized for a linear polarization along the SC principal axes [2]. The result is that the transmitted light at the output will be a checkerboard-like polarization pattern, with alternating orthogonally polarized states (see Fig.8, for $E = 0$). This naturally amounts to a natural 3D orthographic projection, opening the possibility of observing optically the microscopic details of SC cluster dynamics even though it is taking place on the micrometer scale in a full 3D volume [3]. Supporting the main text, Fig. 8 a more detailed phenomenology is reported, where polarization transmission images through the sample are shown for various temperatures below $T_c$ =294K and different external electric fields $E$. The sudden transition at $T_c$−4.5 K evolves into a much richer phenomenology, fully compatible with our hypothesis of an emergent metastable phase. In fact, for a temperature up $T_C - 3.5K$, the SC does not show any more sudden polarization changes. Crossed-polarizer transmission starts to decrease along particular directions, oriented at 45 degrees relative to the crystal principal axes ($E_c$ = 2.81 kV/cm). Despite this, light transmission remains evident in the overall image. Increasing temperature further ($T_C - 2.5K$), SC distortions appear at a lower field, $E_c$=2.5 kV/cm along the inclined paths, analogously to the previous case. As the bias field increases, the dark regions expand along these specific directions until they cover the entire transmitted image at $E_c$= 2.96 kV/cm, analogously to the case at $T_C - 4.5K$.

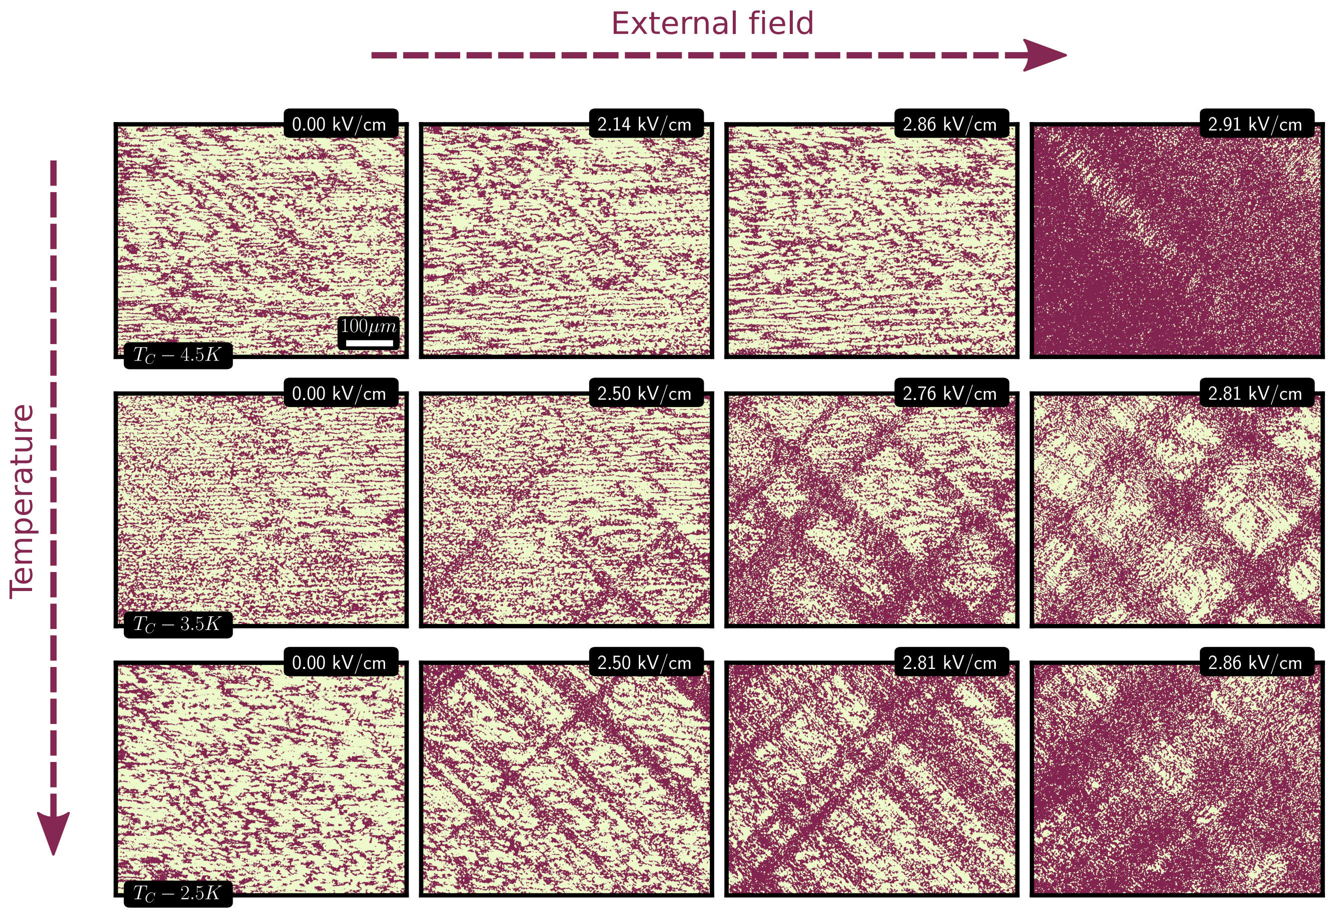


FIG. 8. **Imaging of ferroelectric SC cluster dynamics.** Crossed-polarizer transmission microscopy images in various conditions of temperature and bias electric field.

* pablo.villegas@cref.it

[1] P. Villegas, T. Gili, G. Caldarelli, and A. Gabrielli, Laplacian renormalization group for heterogeneous networks, Nat. Phys. **19**, 445 (2023).
[2] M. Ferraro, D. Pierangeli, M. Flammini, G. Di Domenico, L. Falsi, F. Di Mei, A. Agranat, and E. DelRe, Observation of polarization-maintaining light propagation in depoled compositionally disordered ferroelectrics, Opt. Lett. **42**, 3856 (2017).
[3] L. Falsi, M. Aversa, F. Di Mei, D. Pierangeli, F. Xin, A. J. Agranat, and E. DelRe, Direct observation of fractal-dimensional percolation in the 3d cluster dynamics of a ferroelectric supercrystal, Phys. Rev. Lett. **126**, 037601 (2021).
